# Supplementary material for: From Dialogue to Diagnostic Hypotheses: Evaluating LLM Agents for Psychiatric Assessment
Source: arXiv:2610.07473 source file (2026-11-06)
Supplement: Supplementary file 1 [file appendix.tex]

% Appendix-only layout helpers leave the reviewed main manuscript unchanged.
\makeatletter
\newcommand{\AppendixFigureCaption}[2]{\begingroup\def\@captype{figure}\captionsetup{hypcap=false}\caption{#1}\label{#2}\endgroup}
\newcommand{\AppendixTableCaption}[2]{\begingroup\def\@captype{table}\captionsetup{hypcap=false}\caption{#1}\label{#2}\endgroup}
% Record the physical final page after pending appendix floats have shipped.
\newcommand{\AppendixEnd}{\clearpage\immediate\write\@auxout{\string\newlabel{lastappendixpage}{{}{\number\numexpr\value{page}-1\relax}{}{page.\number\numexpr\value{page}-1\relax}{}}}}
\makeatother
\input{sections/appendix/reader-guide}
\clearpage
\input{sections/appendix/psycpg/section}
\clearpage
\input{sections/appendix/psycidra/section}
\clearpage
\input{sections/appendix/protocol/section}
\clearpage
\input{sections/appendix/simulation-results/section}
\clearpage
\input{sections/appendix/human-results/section}
