# Supplementary material for: From Dialogue to Diagnostic Hypotheses: Evaluating LLM Agents for Psychiatric Assessment
Source: arXiv:2610.07473 source file (2026-11-06)
Supplement: Supplementary file 2 [file confidence.tex]

\subsection{Reported Support and Confidence}
\label{app:human-confidence}
\begin{minipage}{\textwidth}
\centering
\includegraphics[width=\textwidth]{app_e_confidence.pdf}
\AppendixFigureCaption{First-code outcomes by reported category. Green: exact reference matches. Single/crossed hatching: other codes on expert-positive/expert-withheld transcripts. Labels give percentages and counts; withheld reports have no category.}{fig:app-e-confidence}
\label{fig:app-e-confidence-differentials}
\end{minipage}
