# Supplementary material for: From Dialogue to Diagnostic Hypotheses: Evaluating LLM Agents for Psychiatric Assessment
Source: arXiv:2610.07473 source file (2026-11-06)
Supplement: Supplementary file 3 [file diagnostic-content.tex]

\twocolumn[{
\begin{minipage}[t]{.49\textwidth}
\vspace{0pt}
\centering\small
\setlength{\tabcolsep}{3pt}
\input{generated/app_e_codes}
\AppendixTableCaption{Exact reference-code counts on 43 shared expert-positive transcripts. R1: first code; Any: anywhere in the final list. Both diagnosers use the same row denominators.}{tab:app-e-codes}
\end{minipage}\hfill
\begin{minipage}[t]{.49\textwidth}
\vspace{0pt}
\centering\small
\setlength{\tabcolsep}{3pt}
\input{generated/app_e_selfreport_decisions}
\AppendixTableCaption{Final hypotheses issued within each self-reported diagnosis group; the remainder are withheld. Experts use the reconciled reference. Unsure/declined: 3/1; unanswered: 14 absent forms and four skipped answers.}{tab:app-e-selfreport}
\end{minipage}
\vspace{.7em}
\begin{minipage}[t]{.48\textwidth}
Primary codes are reconciled, but full expert lists differ on 15/43 positive transcripts and support ratings on 13/43. Rows with one transcript describe individual cases.
\end{minipage}\hfill
\begin{minipage}[t]{.48\textwidth}
Among 65 participants reporting no professional diagnosis, experts issue 21 hypotheses, Direct 45, and PsyDARA 34. Self-report describes diagnostic history, not an independent assessment of the present transcript.
\end{minipage}
\vspace{.5em}
\input{sections/appendix/human-results/confidence}
\vspace{.7em}
}]

Direct's \emph{low support} means that assigning the diagnosis is unsupported. PsyDARA's \emph{low confidence} denotes a plausible leading hypothesis with unresolved evidence. The labels are ordinal, with different definitions across methods.

\newpage
PsyDARA reports no high-confidence first hypotheses. Its moderate category contains both kinds of disagreement. One of its 40 withheld reports concerns an expert-positive transcript.
