# Supplementary material for: From Dialogue to Diagnostic Hypotheses: Evaluating LLM Agents for Psychiatric Assessment
Source: arXiv:2610.07473 source file (2026-11-06)
Supplement: Supplementary file 4 [file diagnostic-decisions.tex]

\twocolumn[{
\subsection{Diagnostic Decisions and Code Agreement}
\label{app:diagnostic-decisions}
\label{app:human-diagnostic-content}
\label{app:human-confusion}
\label{app:human-paired}
\begin{minipage}{\textwidth}
\centering
\includegraphics[width=\textwidth]{app_e_decision_confusion.pdf}
\AppendixFigureCaption{Whether the AI issues a final hypothesis. Rows show reconciled expert decisions; columns show AI decisions. Cells give counts divided by expert-row totals. Diagnosers process identical transcripts within each interview arm; interview arms contain different participants. A nonempty list counts as issued regardless of code agreement.}{fig:appendix-human-confusion}
\vspace{.8em}
\small\setlength{\tabcolsep}{5pt}
\input{generated/app_e_paired}
\AppendixTableCaption{Paired outcomes on shared transcripts. Both and neither refer to agreement with the expert reference; Direct only and PsyDARA only identify transcripts on which the diagnosers differ. Code endpoints use the 43 expert-positive transcripts.}{tab:appendix-human-paired}
\end{minipage}
\vspace{1em}
}]

The paired counts locate the change in decisions: all 12 gains involve withholding on expert-withheld transcripts, while the one loss is a withheld output on an expert-positive transcript. Changes in reference-code agreement involve fewer transcripts.

\begin{center}\begin{minipage}{\columnwidth}
\centering\small
\setlength{\tabcolsep}{3pt}
\input{generated/app_e_differentials}
\AppendixTableCaption{AI outputs on the 58 transcripts where experts withheld a final diagnosis, grouped by how many reviewers listed at least one differential candidate. Both reviewers listing candidates does not require the same code.}{tab:app-e-differentials}
\end{minipage}\end{center}

\newpage
Differential lists help explain what withholding means. At least one expert retained a possible diagnosis on 34/58 final-withheld transcripts. Eight of the 12 changes from an issued Direct hypothesis to a withheld PsyDARA output occur where only one expert listed a candidate. These possibilities do not change the final reference or the agreement counts.

Adjustment disorder accounts for 22/31 Direct and 13/19 PsyDARA first codes on expert-withheld transcripts. The first code appears in an expert differential in 23/31 and 14/19, respectively: a considered possibility can remain outside the final reference.

\label{app:initial-agreement}
Initial judgments survive for 50 analyzed transcripts (26 Direct, 24 PsyCIRA) in the August~30 archive. Reviewers agreed on issuing a diagnosis in 44/50 and on the first code in 9/12 where both issued one. These unreconciled counts describe only that subset.
