# Supplementary material for: From Dialogue to Diagnostic Hypotheses: Evaluating LLM Agents for Psychiatric Assessment
Source: arXiv:2610.07473 source file (2026-11-06)
Supplement: Supplementary file 5 [file participant-experience.tex]

\twocolumn[{
\subsection{Participant-Reported Experience}
\label{app:experience}
\begin{minipage}{\textwidth}
\centering
\includegraphics[width=\textwidth]{app_e_experience.pdf}
\AppendixFigureCaption{Responses to the six optional experience questions. Categories run from strongly disagree (1) to strongly agree (5); each arm's observed-response denominator is shown. Higher agreement is favorable for the first five items but means greater reported distress for the last. Unanswered items are omitted from the plotted distributions.}{fig:appendix-experience}
\end{minipage}
\vspace{1em}
}]

Agreement that the conversation flowed naturally is less common (20/39 Direct and 25/42 PsyCIRA responses) than agreement that questions were clear (37/39 and 39/41). The item distributions distinguish understandable questions from an easy conversational exchange.

Of the 15 respondents who agreed that distress increased, 11 also agreed that they felt comfortable. Comfort and distress can therefore coexist; combining them into a single satisfaction score would conceal this pattern.

No pre-interview distress score or follow-up establishes how much distress changed or how long it lasted. These responses describe the interaction without establishing clinical benefit or harm.

\newpage
\begin{center}\begin{minipage}{\columnwidth}
\centering\small
\setlength{\tabcolsep}{3pt}
\input{generated/app_e_comfort_distress}
\AppendixTableCaption{Joint comfort and increased-distress responses among 80 participants answering both items. Agreement means ratings 4--5; other responses are 1--3. Counts refer to the same respondents within each row.}{tab:app-e-comfort-distress}
\end{minipage}\end{center}
