# Supplementary material for: From Dialogue to Diagnostic Hypotheses: Evaluating LLM Agents for Psychiatric Assessment
Source: arXiv:2610.07473 source file (2026-11-06)
Supplement: Supplementary file 6 [file participant-flow.tex]

\subsection{Participant Flow and Cohort Composition}
\label{app:human-attrition}
\label{app:participants}
\begingroup
\fontsize{10pt}{12pt}\selectfont

The 101 analyzed interviews each have two expert reviews and reports from both diagnosers. Interview comparisons involve different volunteers; diagnoser comparisons reuse their transcripts.

\par\medskip\noindent\begin{minipage}{\columnwidth}
\centering\small
\setlength{\tabcolsep}{4pt}
\input{generated/app_e_demographics}
\AppendixTableCaption{Demographic counts in the analyzed cohort: 52 Direct and 49 PsyCIRA interviews.}{tab:appendix-demographics}
\end{minipage}\par\medskip

Most volunteers were aged 18--34 (61/101), and 88 held a bachelor's or master's degree. These characteristics describe the recruited sample, not a clinical population.

The platform automatically assigned participants to Direct or PsyCIRA at registration. When enrollment counts were equal, a random tie-break determined the assignment; otherwise, the next registrant entered the underrepresented arm, maintaining balanced enrollment. Assignment did not depend on participant characteristics or investigator selection, and participants could not choose their interview mode.

\newpage
The four excluded safety stops had fewer than six participant responses. Experts excluded eight completed interviews because their content was unrelated to mental-health assessment, including spam and nonclinical exchanges. All eight met the six-response threshold; exclusion concerned relevance, not interview quality or speaking style. Three excluded stops were participant-requested and one model-originated. Both retained stops were model-originated, one per arm.

\par\medskip\noindent\begin{minipage}{\columnwidth}
\centering\small
\setlength{\tabcolsep}{3pt}
\input{generated/app_e_availability}
\AppendixTableCaption{Available evidence in the analyzed cohort. Saved questionnaires may contain unanswered items.}{tab:app-e-availability}
\end{minipage}\par\medskip

\par\medskip\noindent\begin{minipage}{\columnwidth}
\centering\footnotesize
\setlength{\tabcolsep}{2.2pt}
\input{generated/app_e_history}
\AppendixTableCaption{Self-reported history, pooled across 101 participants. Other includes waiting/planning, being under assessment, uncertainty, or refusal; missing denotes an absent answer. Past and current responses remain separate.}{tab:app-e-history}
\end{minipage}\par\medskip

History describes prior care, not an independent diagnostic reference. Questionnaire wording appears in Appendix~\ref{app:protocol}.
\par\endgroup
