# Supplementary material for: From Dialogue to Diagnostic Hypotheses: Evaluating LLM Agents for Psychiatric Assessment
Source: arXiv:2610.07473 source file (2026-11-06)
Supplement: Supplementary file 7 [file quality-safety.tex]

\twocolumn[{
\subsection{Interview Quality and Safety}
\label{app:expert-agreement}
\label{app:quality-agreement}
\label{app:quality-items}
\begin{minipage}{\textwidth}
\centering
\includegraphics[width=\textwidth]{app_e_quality_items.pdf}
\AppendixFigureCaption{Expert ratings by item. Each point averages available reviewers within transcripts, then transcripts within an interview arm; the difference is PsyCIRA minus Direct. AIIE uses a 1--5 scale and CCSS-S a 0--3 scale. CCSS-S item~13 is omitted because only 29/202 reviewer responses are evaluable, with no complete reviewer pairs.}{fig:appendix-quality-items}
\end{minipage}
\vspace{1em}
}]

Question clarity receives high ratings in both arms (4.55 Direct, 4.68 PsyCIRA, out of~5). Empathetic validation (3.34, 3.59), differential exploration (3.46, 3.41), and medical/biological rule-outs (3.57, 3.04) receive lower ratings. These item-level scores identify specific weaknesses that the overall means conceal.

\newpage
Within CCSS-S, empathy receives the lowest mean rating in both arms (1.89 Direct, 2.09 PsyCIRA, out of~3), while nonjudgmental stance is near the scale maximum (2.98 in both). These items distinguish avoiding judgment from demonstrating empathy.

\twocolumn[{
\begin{minipage}{\textwidth}
\centering\small
\setlength{\tabcolsep}{4pt}
\input{generated/app_e_reviewer_descriptive}
\AppendixTableCaption{Each reviewer's mean ratings by interview arm. $\Delta$ is PsyCIRA minus Direct. AIIE and its domains use a 1--5 scale; adapted CCSS-S uses a 0--3 scale. Medical/biological rule-outs is an individual item within diagnostic inquiry.}{tab:appendix-quality-agreement}
\end{minipage}
\vspace{1em}
}]

Both reviewers rate PsyCIRA higher for rapport, interview flow, and overall CCSS-S. Their diagnostic-inquiry differences point in opposite directions ($+0.09$ and $-0.41$). This disagreement occurs on all five inquiry items. For medical/biological rule-outs, Reviewer~1 gives nearly equal arm means (3.79 and 3.82), while Reviewer~2 gives 3.35 for Direct and 2.27 for PsyCIRA. The pooled gap therefore reflects a marked difference in one reviewer's assessment.

AIIE and AISC responses are complete. Of 179 unavailable CCSS-S item responses, 173 concern item~13. We show the remaining items individually and use available responses when calculating transcript means.

\newpage
\begin{center}\begin{minipage}{\columnwidth}
\centering\small
\setlength{\tabcolsep}{3pt}
\input{generated/app_e_safety_by_arm}
\AppendixTableCaption{AISC concerns by interview arm. Either counts a transcript flagged by at least one reviewer; both counts concordant flags. Four other checklist items have no recorded flags.}{tab:app-e-safety}
\end{minipage}\end{center}

\label{app:safety-agreement}
The reviewers both flag a concern on one transcript, and only one reviewer flags a concern on four others. Both crisis-handling concerns occur in PsyCIRA interviews.

Checklist concerns and live stops capture different events. A stop records activation of the intervention mechanism; a checklist flag records a reviewer's judgment about the transcript. Neither the five flagged interviews nor the two analyzed safety stops describe the safety of the 12 excluded ended sessions.
