# Supplementary material for: From Dialogue to Diagnostic Hypotheses: Evaluating LLM Agents for Psychiatric Assessment
Source: arXiv:2610.07473 source file (2026-11-06)
Supplement: Supplementary file 8 [file resources.tex]

\twocolumn[{
\subsection{Latency and Computational Resources}
\label{app:resources}
\begin{minipage}{\textwidth}
\centering
\includegraphics[width=\textwidth]{app_e_latency_distribution.pdf}
\AppendixFigureCaption{Recorded latency in seconds. Each point represents one interview's mean reply interval (left) or one diagnostic report's duration (right). Shading spans the 25th--75th percentiles; the horizontal line marks the median. All observations are retained. The interview arms contain different participants; both diagnosers process the same 101 transcripts.}{fig:app-e-latency-distribution}
\vspace{.8em}
\begingroup
\small
\setlength{\tabcolsep}{7pt}
\input{generated/app_e_tokens}
\AppendixTableCaption{Mean recorded API tokens per interview or diagnostic report, in thousands. Interview accounting uses the complete usage ledger. Cached input is a subset of input and is counted only once in the total. Output includes reasoning tokens where counted by the provider. Totals are calculated before rounding.}{tab:app-e-tokens}
\endgroup
\end{minipage}
\vspace{1em}
}]

Reply intervals run from a participant message's stored timestamp to the next assistant text, including orchestration and persistence overhead. All 1,604 messages have a matched reply (822 Direct, 782 PsyCIRA); the opening greeting is excluded. Median individual-reply intervals are 3.50~s for Direct and 3.98~s for PsyCIRA, indicating a modest difference in typical conversational delay. P95 is 5.99~s and 12.25~s, respectively, with maxima of 68.07~s and 215.47~s. Report generation follows the completed interview and supports subsequent expert review without a real-time response requirement. Its longer duration therefore does not add to chat reply latency. Median report durations are 5.54~s for Direct and 28.53~s for PsyDARA, excluding queue time.

\newpage
Mean recorded token use is 13.1 times higher for PsyCIRA interviews than for Direct interviews, and 8.6 times higher for PsyDARA reports than for Direct reports. The increase primarily reflects repeated input context rather than longer outputs. These API-token ratios do not imply equivalent cost ratios: cached input accounts for 93.8\% of PsyCIRA input and 34.8\% of PsyDARA input and receives discounted pricing. For the same 49 PsyCIDRA participants, the mean recorded interview API cost is USD~0.113. Applying the frozen study-time rates of USD~2.00/0.20/12.00 per million uncached-input/cached-input/output tokens gives an estimated mean report cost of USD~0.050, yielding approximately USD~0.16 per interview and report. This combined estimate excludes hosting and expert labor. The modest absolute model-API cost can justify the additional computation for the intended workflow, which produces an interview and structured report for subsequent expert review.
