# Supplementary material for: From Dialogue to Diagnostic Hypotheses: Evaluating LLM Agents for Psychiatric Assessment
Source: arXiv:2610.07473 source file (2026-11-06)
Supplement: Supplementary file 9 [file section.tex]

\twocolumn[{
\section{Human-Participant Study: Extended Analysis}
\label{app:human-results}
\label{app:feasibility}
\begin{minipage}{\textwidth}
\centering
\includegraphics[width=\textwidth]{app_e_participant_flow.pdf}
\AppendixFigureCaption{Participant flow from registration to the analyzed cohort. Completed and safety-stopped sessions are mutually exclusive. Active sessions had not ended at the registration-ledger cutoff.}{fig:app-e-flow}
\label{tab:appendix-participant-flow}
\end{minipage}
\vspace{1em}
}]


\input{sections/appendix/human-results/participant-flow}
\input{sections/appendix/human-results/quality-safety}
\input{sections/appendix/human-results/diagnostic-decisions}
\input{sections/appendix/human-results/diagnostic-content}
\input{sections/appendix/human-results/participant-experience}
\input{sections/appendix/human-results/resources}
