# Supplementary material for: From Dialogue to Diagnostic Hypotheses: Evaluating LLM Agents for Psychiatric Assessment
Source: arXiv:2610.07473 source file (2026-11-06)
Supplement: Supplementary file 10 [file 02-measures-instruments.tex]

\twocolumn[{
\section{Evaluation Instruments}
\label{app:protocol}
\label{app:evaluation-protocol}
\subsection{Expert evaluation instruments}
\label{app:instruments}
\begin{minipage}{\textwidth}
\begin{minipage}[t]{.48\textwidth}
\paragraph{CCSS-S.}
We used a 12-item adaptation of the CCSS-S to assess clinical communication \citep{maass-2022-ccss-s}. Items 1 and 3 were omitted because they were not applicable to the text-based chat format.

\paragraph{AIIE.}
AIIE distinguishes the clinical evidence elicited by the interviewer from the way the conversation is conducted. Its clinical items address symptom features, impairment, symptom course, and alternative explanations; other domains capture risk recognition, rapport, and interview flow. This design follows clinical-dialogue evaluations that assess history-taking alongside communication and empathy \citep{tu-2025-amie,johri-2025-craft-md}.
\end{minipage}\hfill
\begin{minipage}[t]{.48\textwidth}
\paragraph{AISC.}
AISC checks for safety concerns and violations of the interviewer's assessment role: participant-facing diagnoses or treatment advice, crisis neglect, inappropriate tone, anthropomorphic claims, boundary violations, and unnecessary sensitive-data requests. These review targets reflect health-AI guidance and risks identified for mental-health conversational systems \citep{who-2024-lmm-guidance,lawrence-2024-llm-mental-health-risks}. Binary flags keep an isolated concern visible even when the interview receives favorable quality ratings.

Figures~\ref{fig:app-c-aiie} and~\ref{fig:app-c-aisc} present the complete study-developed forms, including their response options and scoring instructions.
\end{minipage}
\end{minipage}
\vspace{8pt}
\subsection{Participant questionnaires}
\label{app:participant-instruments}
\begin{minipage}{\textwidth}
After the interview, human participants were invited to complete two optional questionnaires on mental health history and interview experience.
\vspace{6pt}

\centering\small
\setlength{\tabcolsep}{4pt}\renewcommand{\arraystretch}{1.15}
\begin{tabularx}{\textwidth}{@{}>{\raggedright\arraybackslash}p{.11\textwidth}>{\raggedright\arraybackslash}X>{\raggedright\arraybackslash}p{.32\textwidth}@{}}
\toprule
Form & Question & Responses \\
\midrule
Mental health history & Have you ever had a specialist mental-health assessment or interview with a psychologist, psychiatrist, or counselor? & Never; previously; currently being assessed; unsure; prefer not to answer. \\
 & Have you ever received psychotherapy or counseling for psychological concerns? & Never; previously; currently; waiting/planning; prefer not to answer. \\
 & Has a mental-health professional ever proposed a psychological or psychiatric diagnosis for you? & No; past diagnosis without current follow-up; current diagnosis/follow-up; assessment without a diagnosis; unsure; prefer not to answer. \\
 & If you wish, give the name of the diagnosis or disorder proposed. & Optional free text; no details of severity, duration, or treatment requested. \\
 & Have you ever taken medication prescribed by a physician or psychiatrist for your mental health? & Never; previously; currently; unsure; prefer not to answer. \\
\midrule
Interview experience & The system's tone was respectful, empathetic, and nonjudgmental. & Each statement: 1, strongly disagree; 2, disagree; 3, neither agree nor disagree; 4, agree; 5, strongly agree. All optional. \\
 & The conversation was natural and fluent, without feeling mechanical or repetitive. & \\
 & The questions were relevant to my situation rather than unrelated or random. & \\
 & Understanding and answering the questions was easy for me. & \\
 & I felt comfortable discussing personal and psychological topics. & \\
 & After the conversation, my discomfort, psychological pressure, or distress increased. & Higher agreement is less favorable for this item. \\
 & Briefly describe any uncomfortable, inappropriate, or unsafe part; what should improve; any other comments. & Three separate optional free-text prompts. \\
\bottomrule
\end{tabularx}
\AppendixTableCaption{Optional participant questionnaires. History responses provide context for the cohort; experience responses describe the interaction. The three free-text prompts are grouped for space.}{tab:app-c-participant-forms}
\end{minipage}
}]
\clearpage
