# Supplementary material for: From Dialogue to Diagnostic Hypotheses: Evaluating LLM Agents for Psychiatric Assessment
Source: arXiv:2610.07473 source file (2026-11-06)
Supplement: Supplementary file 11 [file 03-aiie-form.tex]

\twocolumn[{
\subsection{AI Interview Examination}
\label{app:aiie-form}
\begin{minipage}{\textwidth}
\centering
\includegraphics[width=\textwidth,height=.88\textheight,keepaspectratio]{app_c_aiie_form.pdf}
\AppendixFigureCaption{AIIE: fourteen items with five response anchors, grouped by diagnostic inquiry, risk recognition, rapport, and interview flow.}{fig:app-c-aiie}
\end{minipage}
}]
\clearpage
