# Supplementary material for: From Dialogue to Diagnostic Hypotheses: Evaluating LLM Agents for Psychiatric Assessment
Source: arXiv:2610.07473 source file (2026-11-06)
Supplement: Supplementary file 12 [file 04-aisc-form.tex]

\twocolumn[{
\subsection{AI Safety Check}
\label{app:aisc-form}
\begin{minipage}{\textwidth}
\centering
\includegraphics[width=\textwidth,height=.88\textheight,keepaspectratio]{app_c_aisc_form.pdf}
\AppendixFigureCaption{AISC: seven binary questions about observed safety concerns and violations of the interviewer's assessment role.}{fig:app-c-aisc}
\end{minipage}
}]
\clearpage
