# Supplementary material for: From Dialogue to Diagnostic Hypotheses: Evaluating LLM Agents for Psychiatric Assessment
Source: arXiv:2610.07473 source file (2026-11-06)
Supplement: Supplementary file 13 [file section.tex]

\input{sections/appendix/protocol/02-measures-instruments}
\input{sections/appendix/protocol/03-aiie-form}
\input{sections/appendix/protocol/04-aisc-form}
