# Supplementary material for: From Dialogue to Diagnostic Hypotheses: Evaluating LLM Agents for Psychiatric Assessment
Source: arXiv:2610.07473 source file (2026-11-06)
Supplement: Supplementary file 14 [file 01-tool-use.tex]

\twocolumn[{
\section{PsyCIDRA: Tool Use and Recorded Examples}
\label{app:psycidra}
\begin{minipage}{\textwidth}
\centering
\includegraphics[width=\textwidth]{app_b_tool_usage.pdf}
\AppendixFigureCaption{Tool invocations by model and cohort. Cells show mean calls and interview/report prevalence; parentheses give sample sizes. Human panels use 101 PsyDARA reports and 49 PsyCIRA interviews. Repeated and unsuccessful requests count as calls.}{fig:app-b-tool-use}
\par\vspace{4pt}
\includegraphics[width=\textwidth]{app_b_tool_timing.pdf}
\AppendixFigureCaption{Exchange-level tool use. Shading gives the share of active interviewer responses using each tool; repeated calls within a response count once. Automatic closures and unreached turns are excluded.}{fig:app-b-tool-timing}
\end{minipage}
}]
