# Supplementary material for: From Dialogue to Diagnostic Hypotheses: Evaluating LLM Agents for Psychiatric Assessment
Source: arXiv:2610.07473 source file (2026-11-06)
Supplement: Supplementary file 15 [file 02-analysis.tex]

\twocolumn[{
\begin{minipage}{\textwidth}
\centering
\includegraphics[width=\textwidth]{app_b_notepad.pdf}
\AppendixFigureCaption{One recorded PsyCIRA notepad update in a GPT-5.6 Terra simulated interview at exchange 7. The panels show the state immediately before the call and its returned state; the arrow links the latest patient reply to the actions in that call. Text is abridged and translated into English.}{fig:app-b-notepad}
\end{minipage}
}]
\subsection{Observed tool use}
\label{app:tool-use}
\label{app:tool-timing}
PsyDARA consults disorder references in nearly all simulated reports. PsyCIRA's tool use varies more: GPT-5.6 Luna makes 7.15 skill requests per interview, compared with 0.43 for GPT-5.6 Terra (Figure~\ref{fig:app-b-tool-use}). These counts cannot establish a relationship with diagnostic performance. They show different model behaviors under shared agent instructions and tools; reasoning settings also differ, so the comparison is descriptive.

GPT-5.6 Terra retrieves references most often at exchange 2 in both simulated cohorts, while its note updates span the interview. GPT-5.6 Luna's skill requests recur across early and middle exchanges (Figure~\ref{fig:app-b-tool-timing}).

\subsection{PsyCIRA notepad tool}
\label{app:notepad-example}
Agent memory can retain observations, reflections, or feedback to guide later decisions \citep{park-2023-generative-agents,shinn-2023-reflexion,hu-2025-hiagent}. PsyCIRA's notepad applies this principle within one interview: keep salient findings and follow-up priorities accessible, while allowing earlier interpretations to change as evidence develops.

Its five fields hold salient evidence, covered topics, unresolved issues, provisional hypotheses, and a plan for inquiry. Entries have persistent identifiers. PsyCIRA can read the notes or submit one ordered batch of add, edit, and delete actions. New entries receive identifiers; edits and deletions target existing ones. The tool returns an action summary and the full updated notepad, so an immediate separate read is unnecessary. Instructions call for updates when the case summary or plan materially changes and favor consolidating notes.

We include one recorded call in Figure~\ref{fig:app-b-notepad} to clarify the interface, showing the triggering patient reply and the notepad immediately before and after the update.
