# Supplementary material for: From Dialogue to Diagnostic Hypotheses: Evaluating LLM Agents for Psychiatric Assessment
Source: arXiv:2610.07473 source file (2026-11-06)
Supplement: Supplementary file 16 [file 03-report-example.tex]

\subsection{PsyDARA diagnosis report structure}
\label{app:evidence-interface}
The report begins with data sufficiency and a problem representation. Evidence items record each finding's state, source, timeframe, diagnostic salience, and relevance, keeping explicit denials distinct from unassessed information. Alternative explanations and a ranked ICD-11 differential follow. Each candidate records supporting and contradictory evidence, unresolved requirements, a support level, and a clinical judgment.

A diagnostic synthesis explains the ranking, followed by key uncertainties and a separate safety assessment. The final field contains zero to three ranked hypotheses with ICD-11 names, codes, and confidence levels; an empty list indicates withholding. Candidate support and final confidence express evidential judgments at different stages.

We include one recorded report in Figure~\ref{fig:app-b-report} to clarify this structure.

\clearpage
\begin{figure*}[p]
\centering
\includegraphics[width=.99\textwidth]{app_b_report.pdf}
\caption{A recorded PsyDARA report for the simulated profile in Figure~\ref{fig:appendix-patient-profile}. Four of eight findings are displayed; narrative and reasoning are abridged in English. Candidate ranks, codes, evidence states, support levels, and final confidence are retained.}
\label{fig:app-b-report}
\end{figure*}
