# Supplementary material for: From Dialogue to Diagnostic Hypotheses: Evaluating LLM Agents for Psychiatric Assessment
Source: arXiv:2610.07473 source file (2026-11-06)
Supplement: Supplementary file 17 [file section.tex]

\input{sections/appendix/psycidra/01-tool-use}
\input{sections/appendix/psycidra/02-analysis}
\input{sections/appendix/psycidra/03-report-example}
