# Supplementary material for: From Dialogue to Diagnostic Hypotheses: Evaluating LLM Agents for Psychiatric Assessment
Source: arXiv:2610.07473 source file (2026-11-06)
Supplement: Supplementary file 18 [file 01-positioning-design.tex]

\subsection{Related approaches and design goals}
\label{app:literature-simulation}

A patient simulator is part of the measurement instrument: its responses determine the evidence available to an interviewer and the effort required to elicit it. Useful simulation therefore depends on more than fluency or agreement with a diagnostic label. It must preserve clinical content, portray a plausible person, and expose information in ways that make interviewing meaningful. Prior work addresses these requirements from several complementary directions. Table~\ref{tab:appendix-simulation-literature} maps representative approaches by their source material, construction method, clinical scope, and intended use. This is a targeted comparison, rather than a systematic review or a ranking of results across different tasks.

\paragraph{Expert-authored mental-health patients.}
PATIENT-$\psi$ uses 106 cognitive models manually constructed by two clinical psychologists, drawing on summarized therapy transcripts, with six conversational styles \citep{wang-2024-patient-psi}. Its target is CBT formulation and professional training, rather than diagnosis across a broad psychiatric case collection. Roleplay-doh similarly places expert knowledge at the center: counselors author scenarios and turn feedback into explicit simulation principles, with response checking and revision to improve adherence \citep{louie-2024-roleplay-doh}. These approaches show why a clinically meaningful patient needs a perspective and behavioral constraints, and why an LLM's apparent naturalness is insufficient on its own. Their expert authoring process also serves a different purpose from automatically transforming an existing collection of diagnosis-labelled records.

\paragraph{Psychiatric assessment and evolving behavior.}
PSYCHE generates profile, history, and mental-status behavior for seven disorder conditions and evaluates psychiatric assessment agents \citep{lee-2025-psyche}. Breaking the Stigma uses depression-oriented user profiles and stigma templates to study symptom probing \citep{cao-2025-stigma}. AnnaAgent adds emotion changes, complaint progression, and memory across counseling sessions \citep{wang-2025-annaagent}; PUPPET uses expert-defined symbolic rules to govern mental-state transitions in CBT, motivational interviewing, and crisis-hotline scenarios \citep{xu-2026-puppet}. These studies make important dimensions of psychiatric interaction explicit. Their different emphases---diagnosis-conditioned construction, stigma, longitudinal change, and intervention-dependent state---also show that simulation controls should be chosen for the research question, rather than treated as a single measure of realism.

\paragraph{Record-grounded simulation and controlled personas.}
PatientSim builds 170 clinical profiles from MIMIC records and combines them with 37 persona configurations covering personality, language proficiency, recall, and confusion \citep{kyung-2025-patientsim}. Its five diagnoses cover myocardial infarction, pneumonia, urinary tract infection, intestinal obstruction, and stroke. The emergency-department setting distinguishes clinical grounding from how a patient communicates that information. The more recent Patients With Personality preprint uses HEXACO traits and selective access to fact groups to control behavior and reduce oversharing in general clinical encounters \citep{schlager-2026-pwp}. Personality and inquiry-dependent disclosure thus have direct precedents. PsyCPG's contribution is their integration with psychiatric case transformation, explicit provenance, cohort-level sampling, an expert contextual resource, and source-preserving risk and interaction controls.

\paragraph{Evidence from clinical education journals.}
Medical-education studies provide a further perspective on scale and validation. Cook et al. combine two manually written base scenarios with preference variations to support clinical reasoning and feedback; their 60 evaluated conversations should not be read as 60 independently authored patients \citep{cook-2025-virtual-patients}. Garc\'{i}a-Torres et al. instantiate 13 written psychopathology cases as virtual patients for student interviewing and diagnostic practice, with educator and psychologist validation \citep{garcia-torres-2025-vsp}. These studies complement NLP benchmarks by examining educational use and the quality of portrayal. Their evaluation settings also reinforce the need to distinguish the number of source cases, profile configurations, interactions, and human judgments.

\begin{table*}[t]
\centering\small
\setlength{\tabcolsep}{4pt}
\renewcommand{\arraystretch}{1.13}
\begin{tabularx}{\textwidth}{@{}>{\raggedright\arraybackslash}p{.19\textwidth}>{\raggedright\arraybackslash}p{.15\textwidth}>{\raggedright\arraybackslash}p{.22\textwidth}>{\raggedright\arraybackslash}p{.20\textwidth}>{\raggedright\arraybackslash}X@{}}
\toprule
Work & Case/profile basis & Construction & Clinical scope & Primary use \\
\midrule
PATIENT-$\psi$ \citeyearpar{wang-2024-patient-psi} & 106 cognitive models & Psychologist-authored, transcript-informed & CBT formulation & Therapist training \\
\addlinespace
Roleplay-doh \citeyearpar{louie-2024-roleplay-doh} & 25 scenarios & Counselor-authored; elicited principles & Counseling concerns & Counseling practice \\
\addlinespace
Breaking the Stigma \citeyearpar{cao-2025-stigma} & D$^4$ profiles; 10 stigma templates & Existing profiles plus authored templates & Depression severity, including non-depression & Symptom probing \\
\addlinespace
PSYCHE \citeyearpar{lee-2025-psyche} & 7 disorder conditions; $N$ NR & Diagnosis-conditioned LLM generation & Mood, anxiety, OCD, PTSD & Assessment-agent evaluation \\
\addlinespace
PatientSim \citeyearpar{kyung-2025-patientsim} & 170 clinical profiles & MIMIC extraction plus persona controls & 5 emergency diagnoses & History taking / differential diagnosis \\
\addlinespace
PUPPET \citeyearpar{xu-2026-puppet} & 3 training scenarios; $N$ NR & Expert rules plus LLM responses & CBT, motivational interviewing, crisis support & Standardized-patient training \\
\addlinespace
Garc\'{i}a-Torres et al. \citeyearpar{garcia-torres-2025-vsp} & 13 cases / patients & Written cases instantiated with LLMs & Psychopathology teaching cases & Student interviewing \\
\addlinespace
Patients With Personality \citeyearpar{schlager-2026-pwp} & 22 actor encounters & Existing case profiles plus trait/disclosure controls & General clinical encounters & Simulator realism / control \\
\addlinespace
PsyCPG (this study) & 320 selected; 212 accepted & Case-based LLM generation and validation & 63 ICD-11 codes in 16 groups & Controlled psychiatric assessment \\
\bottomrule
\end{tabularx}
\caption{A map of patient-simulation approaches. Counts retain their reported units; source cases, cognitive models, templates, and generated conversations are not interchangeable. $N$ NR denotes no distinct profile-corpus count in the material reviewed. PSYCHE and Patients With Personality are cited as preprints. Construction identifies the main authoring route, rather than implying that any pipeline is free of human design. Clinical scope and intended use differ, so the table provides positioning rather than a performance comparison.}
\label{tab:appendix-simulation-literature}
\end{table*}

\subsubsection{From prior work to design objectives}
The literature and our experimental needs led to six design goals. We wanted a simulator suitable for cohort-scale psychiatric assessment, with faithful clinical evidence, varied patient behavior, and explicit control over contextual and interaction demands.

\paragraph{1. Preserve the case's clinical evidence.}
A generated patient should retain the case's clinically important facts, relevant negatives, severity, time course, and uncertainty. Any elaboration must remain compatible with that evidence and distinguishable from source-supported information. Record-grounded simulation motivates treating clinical fidelity as a prerequisite for useful portrayal \citep{kyung-2025-patientsim}.

\paragraph{2. Make disclosure depend on the interview.}
Unprompted oversharing is a documented realism problem in LLM patient simulation \citep{schlager-2026-pwp}. We wanted evidence to emerge through relevant inquiry, with disclosure reflecting the question, sensitivity, and patient perspective. The patient should express plausible uncertainty, reluctance, and limited insight, without presenting clinician-only information as personal knowledge.

\paragraph{3. Support reproducible personality diversity.}
The goal was a cohort with deliberate personality variation, rather than reliance on incidental differences between generated cases. Its intended personality mix should be configurable and reproducible, independently of diagnosis, while supporting varied communication, cooperation, and responses to stress without changing the underlying clinical evidence.

\paragraph{4. Adapt sociocultural context with local expertise.}
Culture shapes expressions of distress, help-seeking, and the patient--clinician relationship, and cultural assessment can alter diagnostic interpretation \citep{lewis-fernandez-2014-cultural-formulation,adeponle-2012-cultural-formulation}. These influences vary across settings and individuals. LLM studies also document Western cultural bias and uneven alignment with underrepresented personas and sensitive social values \citep{naous-2024-cultural-bias,alkhamissi-2024-cultural-alignment}. Sociocultural portrayal should therefore be adaptable with local expertise, reflect individual variation, and avoid unsupported assumptions about identity or beliefs.

\paragraph{5. Control clinical risk and interaction challenges separately.}
Clinical risk must remain grounded in the source case, including its time course. Interaction difficulty should be a separate, configurable dimension: challenges such as interruption or pressure for certainty must remain compatible with the patient and bounded in intensity, without inventing symptoms, risk, or clinical history.

\paragraph{6. Require convincing portrayal and accessible evidence.}
The simulator should portray a convincing patient while keeping clinical evidence accessible through plausible interviewing. Fidelity, disclosure, behavior, and authenticity therefore all mattered, as multidimensional simulation evaluations also emphasize \citep{kyung-2025-patientsim,louie-2024-roleplay-doh}. Fluent presentation or easy diagnostic-label recovery alone would not establish a useful simulator.
