# Supplementary material for: From Dialogue to Diagnostic Hypotheses: Evaluating LLM Agents for Psychiatric Assessment
Source: arXiv:2610.07473 source file (2026-11-06)
Supplement: Supplementary file 19 [file 02-generation-pipeline.tex]

\subsection{Generation, validation, and acceptance}
\label{app:psycpg-generation}
\label{app:profile-preparation}

PsyCPG separates preparation, narrative synthesis, and validation so that each stage has a defined purpose and access to the information it needs. Figure~\ref{fig:appendix-profile-pipeline} shows the stages and the information passed between them. The three preparation calls run in parallel without receiving one another's outputs. All generation-stage LLM calls in this study use Terra with medium reasoning. A profile that passes its first validation requires five logical LLM calls: three preparation calls, one synthesis call, and one validation call. One revision and revalidation increase this to seven; operational retries are separate. The following description traces a case through this procedure.

\begin{figure*}[p]
\centering
\includegraphics[width=\textwidth]{appendix_profile_pipeline.pdf}
\caption{PsyCPG generation pipeline. Shared badges track inputs through three preparation calls, narrative synthesis, validation and extraction, and acceptance. Restricted views define the information available to each stage. Warning-only candidates can undergo one revision and revalidation; initial errors do not enter this branch. Five logical LLM calls produce a clean profile, or seven if revision is attempted. The frozen specification retains audit information, while only its role-play view enters the patient prompt. All reported cohorts use ready profiles.}
\label{fig:appendix-profile-pipeline}
\end{figure*}

\paragraph{Source case and clinical reference.}
The clinical input is a case record with its assigned diagnosis, accompanied by a normalized ICD-11 reference containing the disorder definition and diagnostic requirements. MentalDx Bench supplies the deidentified records and psychiatrist-assigned labels used here \citep{sun-2026-mentalseek-dx}. Of its 712 records, 698 have the reference material required by the generator; 14 share a code whose reference is incomplete. This eligibility check concerns available inputs, rather than the clinical validity of the excluded records.

The case remains authoritative about the person's symptoms, history, timing, and circumstances. The reference helps the generator preserve clinically meaningful relationships and helps the validator identify missing or contradictory evidence. It does not license completing a textbook presentation by inventing facts. For example, an undocumented exclusion can remain unassessed even when the reference identifies it as relevant. Cases enter disjoint study cohorts before generation, and personality controls are prepared for each full selected cohort before acceptance filtering.

\paragraph{Cohort-level personality sampling.}
Personality diversity is designed across a cohort rather than left to independent narrative generations. For each Big Five domain, a randomized Latin hypercube divides the 0--100 range into as many strata as there are selected cases and samples one value from each stratum. This covers the intended trait range without requiring an LLM to decide which patients should be outgoing, reserved, cooperative, or guarded. Iman--Conover rank reordering \citep{iman-1982-rank-correlation} then approximates the domain-correlation structure reported for the BFI-2 Study 3 adult Internet sample \citep{soto-2017-bfi2}, while preserving each domain's sampled values. Stable case-identifier order and seeds 7, 8, and 9 determine assignments for evaluation, simulator validation, and held-out test, respectively.

The five controls are extraversion, agreeableness, conscientiousness, negative emotionality, and open-mindedness. They are sampled independently of case content and diagnosis: social withdrawal, for example, is not used to infer a stable personality trait. The values are synthetic locations within the sampling model, not administered BFI-2 scores or established population percentiles. Their purpose is designed variation in a simulated cohort. The adult correlation reference does not establish age-specific personality validity, and quality filtering can alter the accepted subset's original coverage.

\paragraph{Personality interpretation.}
The first preparation call receives only the five trait values and translates their combination into general Persian behavioral prose. It describes tendencies in communication, cooperation, organization, responses to stress, and flexibility. Keeping the clinical case out of this call prevents personality interpretation from becoming a second source of symptoms or biography. A reserved disposition can shape how a patient answers; it cannot create a social-anxiety history. The output guides narrative synthesis, where these tendencies must remain compatible with the case.

\paragraph{Sociocultural selection.}
The second preparation call receives the case, diagnostic reference, and a compact index of the sociocultural catalogue. The research psychologist authored 195 components across 16 domains for this study's context, including ways of expressing distress, privacy and reputation, family involvement, help-seeking, and sources of support. The selector chooses two to five distinct components and gives a case-relevant rationale. It sees identifiers, headings, and applicability hints; the full descriptions are then retrieved directly from the catalogue. The LLM therefore chooses among defined contextual possibilities rather than inventing each component's meaning.

Synthesis receives these descriptions as optional guidance. A component may shape interpretation or communication, but its selection does not establish a cultural identity or social circumstance as true of that person. Unsupported ethnicity, religion, disability, and other sensitive identity assumptions are prohibited. The catalogue supplies contextual possibilities, rather than classifying patients demographically. For another sociocultural setting, we would revise its content and applicability guidance with relevant experts, adapt the compatible configuration, and reassess the resulting portrayals. Translating the present catalogue alone would not establish suitability. These restrictions reduce opportunities for unsupported portrayal, but their fairness has not been empirically evaluated.

\paragraph{Source-grounded safety assessment.}
The third preparation call assesses self-harm, harm to others, and vulnerability or abuse. A positive assessment requires explicit qualifying source evidence, retaining whether the concern is recent, current, imminent, ongoing, or temporally unspecified. Diagnosis and personality cannot create a risk state. Synthesis must also avoid softening a documented concern or turning a remote, resolved event into a current crisis. The assessment remains a separate constraint throughout generation and role-play.

For these three domains, the simulator uses a closed-world policy: source silence or clearly remote, resolved history produces a negative current-domain assessment. Historical information may remain in the profile. A negative domain prohibits invented risk and requires a consistent negative response about the controlled current risk state when asked directly, while preserving documented remote history. It does not require unsolicited denials. This policy defines a controlled experimental patient's behavior, rather than a clinical rule for interpreting absent documentation. Outside these domains, unspecified information remains unknown. Configuring safety exposure means selecting source-supported cases and domain or timing quotas; it does not mean attaching arbitrary risk to an otherwise incompatible case.

\paragraph{Narrative synthesis.}
The builder combines the case, clinical reference, trait values, personality prose, selected contextual descriptions, and safety guidance into a coherent Persian patient narrative. Its task is to translate clinical documentation into a person who can speak about experiences. Explicit clinical facts, consequential negations, and their uncertainty and temporal relationships remain authoritative. Diagnosis-informed elaboration may supply compatible subjective experience or functional impact, but cannot introduce an episode, precise duration, severe symptom, or exclusion merely to improve diagnostic fit. Nonclinical character development can make the portrayal more individual, but cannot supply diagnostic or safety evidence.

Clinical records may also contain clinician-only observations and interpretations. The fact ledger and disclosure controls distinguish these from what the patient knows and can express.

\paragraph{Validation and structured extraction.}\label{app:profile-validation}
A separate validation context receives the original case, diagnostic reference, safety assessment, and candidate narrative. It does not receive personality prose or cultural-selection rationale. The validator checks fidelity and coherence while extracting demographics, a typed fact ledger, compatible interaction challenges, and diagnostic-requirement coverage. Requirements are linked to ledger evidence as supported, unassessed, or in conflict with the source. An unknown routine exclusion need not become a fabricated negative finding; a contradicted defining feature or unresolved prominent alternative can instead produce a diagnostic-fidelity error.

Checks address the whole candidate: whether additions exceed their permitted role, whether the narrative contradicts the case, and whether safety remains consistent with its prior assessment. The validator uses the same backbone as generation, so a separate context provides procedural separation rather than independent clinical adjudication. An additional automated scan checks patient-facing content for the source code, supplied and canonical diagnostic names, and ``ICD-11,'' accounting for Unicode and Persian orthographic variation. This limits explicit answer leakage, but cannot remove every semantic clue, particularly when diagnosis-informed elaboration makes a presentation clearer.

\paragraph{One revision and an acceptance gate.}
No identified problems yields \emph{ready}; warnings alone yield \emph{needs review}; any error yields \emph{error}. Initial error cases do not enter correction. Warning-only candidates receive one targeted revision using the preceding narrative, reference, safety assessment, and validator extraction. This call does not revisit the raw source or original personality and cultural preparation inputs. The revised narrative is then validated against the original source and checked again for label leakage. There is no further automatic repair cycle.

This bounded procedure makes unsuccessful generation visible. The reported cohorts admit only final ready profiles; the workflow's option to include manually reviewed candidates was not used. Accepted profiles are then frozen with their experiment assignments. The specification retains narrative and structured controls alongside source and generation provenance for auditing; a restricted view supplies the role-playing patient.
