# Supplementary material for: From Dialogue to Diagnostic Hypotheses: Evaluating LLM Agents for Psychiatric Assessment
Source: arXiv:2610.07473 source file (2026-11-06)
Supplement: Supplementary file 20 [file 03-profile-roleplay.tex]

\subsection{Profile representation and role-play boundaries}
\label{app:fact-contract}
\label{app:roleplay-boundaries}

The accepted profile combines a narrative, a fact ledger, and behavioral constraints. The narrative supplies a coherent perspective; each fact records its content, type, timeframe, provenance, and disclosure condition. Provenance distinguishes source evidence, limited diagnostic elaboration, and nonclinical characterization. Clinician-only information remains distinct from patient knowledge. Four disclosure levels permit volunteering, topic-relevant disclosure, disclosure after a direct question, or initial withholding of sensitive information. They establish when a fact may be expressed, without requiring immediate or exhaustive disclosure. The patient must maintain continuity, uncertainty, and plausible insight as the interview develops.

Safety guidance preserves documented risk separately from optional interaction challenges. A seeded scheduler assigns at most one case-compatible challenge, with an earliest eligible turn and activation limit; eight evaluation and 16 held-out profiles receive one. Challenges require a natural conversational opportunity from turn four and cannot introduce symptoms, risk, or history. Most allow one activation without repetition; diagnosis-certainty pressure and interview refusal permit one repetition if ignored. Disclosure and challenge limits are prompt-based controls, so assignment does not establish compliance or activation in dialogue.

Role-play uses the frozen narrative, demographics, traits, ledger content and disclosure conditions, safety guidance, and assigned challenge. The raw case, diagnostic reference, validation findings, audit identifiers, provenance labels, and unselected challenge candidates remain outside the patient prompt. Hash and assignment checks verify that comparisons use the intended character and instructions, although interviewers elicit different conversations. Figure~\ref{fig:appendix-patient-profile} illustrates a retained held-out profile, with abridged English translations of its narrative and four of its nine facts.

\begin{figure*}[p]
\centering
\includegraphics[width=\textwidth]{appendix_patient_profile.pdf}
\caption{A retained PsyCPG patient profile. English translations show abridged narrative excerpts and four of nine ledger facts; ellipses mark omissions. Demographics, traits, fact annotations, safety assessments, and interaction controls retain the frozen specification. The radar shows synthetic controls on a 0--100 scale, not clinical test scores. Audit identifiers and provenance labels remain outside the patient prompt. The assigned response to perceived dismissal is eligible from turn four at a natural opportunity, with at most one activation and no repetition.}
\label{fig:appendix-patient-profile}
\end{figure*}
