# Supplementary material for: From Dialogue to Diagnostic Hypotheses: Evaluating LLM Agents for Psychiatric Assessment
Source: arXiv:2610.07473 source file (2026-11-06)
Supplement: Supplementary file 21 [file 04-cohort-analysis.tex]

\clearpage
\twocolumn[{
\begin{minipage}{\textwidth}
\subsection{Generated cohorts and quality-gate selection}
\label{app:cohort-construction}
\label{app:psycpg-cohort-analysis}

{
\centering\small\setlength{\tabcolsep}{5pt}
\begin{tabular}{lrrrrrrr}
\toprule
Cohort & Selected & Ready & Review & Error & Ready codes & Safety present & Female / male \\
\midrule
Simulator validation & 120 & 78 & 14 & 28 & 51 & 23/78 & 46/32 \\
Evaluation & 80 & 53 & 9 & 18 & 25 & 11/53 & 27/26 \\
Held-out test & 120 & 81 & 12 & 27 & 50 & 38/81 & 36/45 \\
\midrule
Portfolio & 320 & 212 & 35 & 73 & 63 & 72/212 & 109/103 \\
\bottomrule
\end{tabular}
\AppendixTableCaption{Generation outcomes and characteristics of accepted profiles. Ready rates are 65.0\%, 66.3\%, and 67.5\% for simulator validation, evaluation, and held-out testing, respectively. The portfolio contains 63 distinct accepted codes; cohort-level code counts overlap. Safety and gender columns describe accepted profiles. Gender is extracted from the profile rather than balanced to represent a population.}{tab:appendix-cohort-yield}
}
\medskip
{
\centering
\includegraphics[width=.94\textwidth]{app_a_cohorts.pdf}
\AppendixFigureCaption{Diagnostic composition after the quality gate. Cells count accepted profiles in each cohort; bars show pooled accepted/selected counts within each diagnostic category. Empty cells identify categories absent from a retained cohort. Selection and retention therefore both determine the case mix used in subsequent experiments.}{fig:app-a-cohort-composition}
}
\end{minipage}
}]
\paragraph{Retention changes the clinical mixture.} The disjoint cohorts are selected before generation. Validation and held-out testing use seeded category quotas and round-robin code sampling, allocating half the cases to the three emphasized groups. All ready evaluation and held-out profiles enter comparisons; 30/78 validation profiles enter expert review. The gate retains 212/320 profiles, including 16 recovered after revision. Retention differs between mood (36/76) and obsessive-compulsive or related cases (38/40), leaving different evaluation and held-out mixtures (Figure~\ref{fig:app-a-cohort-composition}). Aggregate comparisons therefore reflect case mix as well as source cases; these distributions do not estimate prevalence.

\clearpage
\twocolumn[{
\begin{minipage}{\textwidth}
{
\centering
\includegraphics[width=.92\textwidth]{app_a_profile_controls.pdf}
\AppendixFigureCaption{Fact provenance, disclosure, and ledger size in accepted profiles. Bar percentages use the fact denominators shown at the right; profiles with larger ledgers contribute more. The footer reports facts per accepted profile, with IQR given as the 25th--75th percentiles. These are stored specifications, not observed disclosure behavior.}{fig:app-a-profile-controls}
}
\medskip
{
\centering
\includegraphics[width=.92\textwidth]{app_a_traits.pdf}
\AppendixFigureCaption{Big Five controls after acceptance. Dots show cohort medians and segments the interquartile ranges on the shared 0--100 scale. Filtering can change the assigned cohort balance. These synthetic controls are not measured patient personality scores.}{fig:app-a-retained-traits}
}
\end{minipage}
}]
\paragraph{Evidence requires elicitation.} Only 404/2,480 facts allow spontaneous disclosure; 365 are clinician-only (Figure~\ref{fig:app-a-profile-controls}). The ledger separates patient knowledge from the wider record. Provenance remains validator-assigned; small clinical additions can matter, and accepted cases retain unresolved diagnostic information.

\paragraph{Coverage remains uneven.} Only three accepted profiles are aged 45 or older. Greater safety exposure in held-out testing (38/81) than evaluation (11/53) complicates safety-stop comparisons. Personality and disclosure controls specify intended behavior; expert interviews assess its expression.
