# Supplementary material for: From Dialogue to Diagnostic Hypotheses: Evaluating LLM Agents for Psychiatric Assessment
Source: arXiv:2610.07473 source file (2026-11-06)
Supplement: Supplementary file 22 [file 05-validation-protocol.tex]

\subsection{Simulator-validation protocol and MH-SPQF}
\label{app:psycpg-validation-protocol}

Two psychologists interview 30 validation cases selected with seeded diagnostic and safety quotas (29 codes; nine safety-present cases). Each case appears as raw-case role-play and a PsyCPG patient, yielding 60 interviews with identical Terra and reasoning settings and a 16-exchange ceiling. Each expert conducts 15 interviews per condition and sees one version per case; the other expert sees its counterpart. Experts are blinded to condition, source case, and reference diagnosis, recording hypotheses before source revelation for fidelity assessment.

The study-specific Mental Health Simulated Patient Quality Form (MH-SPQF) was developed with psychology experts. Q1--Q2 separate source fidelity and clinical/temporal coherence from fluent presentation \citep{kyung-2025-patientsim,louie-2024-roleplay-doh}; Q3--Q5 assess individualized character, patient-like communication, and emotional/behavioral realism \citep{wang-2024-patient-psi}. Q6 examines disclosure, uncertainty, and insight, addressing oversharing \citep{schlager-2026-pwp}; Q7 assesses interactional responsiveness \citep{louie-2024-roleplay-doh}; Q8 assesses authenticity in the sociocultural setting of the encounter \citep{lewis-fernandez-2014-cultural-formulation}. Q9 retains a separate overall-authenticity judgment. Five binary flags expose contradiction, unsupported clinical facts, unrealistic disclosure/insight, out-of-role expression, and cultural implausibility beyond average ratings. Compatible nonclinical enrichment is permitted. Figure~\ref{fig:app-a-mh-spqf} reproduces the form, which has not undergone psychometric validation.

% Begin the scoring paragraph in the second column.
\newpage
The core score averages available Q1--Q8 ratings (1--5); N/A is missing. One PsyCPG interview lacks Q2/Q3, leaving 29 pairs for those items and 30 for core scores. PsyCPG-minus-raw-case differences receive equal weight across reviewer-assignment strata; percentile 95\% intervals use 20,000 within-stratum case resamples (seed 20261005). Intervals are pointwise and conditional on these reviewers. A sensitivity analysis standardizes each expert's core ratings using their mean and sample standard deviation. Each transcript has one reviewer, so same-transcript inter-rater reliability cannot be estimated. Exact source-code recovery, first or anywhere in the diagnostic list, separately assesses evidence accessibility.

\input{sections/appendix/psycpg/mh-spqf}
