# Supplementary material for: From Dialogue to Diagnostic Hypotheses: Evaluating LLM Agents for Psychiatric Assessment
Source: arXiv:2610.07473 source file (2026-11-06)
Supplement: Supplementary file 23 [file 06-validation-results.tex]

\clearpage
\twocolumn[{
\begin{minipage}{\textwidth}
\subsection{Expert validation results}
\label{app:psycpg-validation-results}

{
\centering
\includegraphics[width=.90\textwidth]{app_a_validation_effects.pdf}
\AppendixFigureCaption{Case-paired MH-SPQF differences. Dots give equally weighted reviewer-assignment stratum means; segments give pointwise percentile bootstrap 95\% intervals. Positive values favor PsyCPG; Q9 is excluded from the core score.}{fig:app-a-validation-effects}
}
\medskip
{
\centering
\includegraphics[width=.90\textwidth]{app_a_validation_flags.pdf}
\AppendixFigureCaption{MH-SPQF flags in 30 interviews per condition. Flags can co-occur; zero counts do not establish that a failure is impossible.}{fig:app-a-validation-flags}
}
\medskip
{
\centering\small
\input{generated/app_a_diagnosis_pairs}
\AppendixTableCaption{Exact source-code agreement across 30 pairs. Gains/losses denote matches under PsyCPG/raw-case only.}{tab:app-a-diagnosis-pairs}
}
\end{minipage}
}]

\paragraph{Improved portrayal, with remaining failures.} PsyCPG's largest gains concern communication, character, and disclosure (Figure~\ref{fig:app-a-validation-effects}). The core score increases by +0.67 (95\% interval 0.35--1.00), with a consistent direction after within-expert standardization. Source fidelity has a smaller estimated gain from a high baseline (4.37); its interval and that for cultural authenticity touch zero. Any flag falls from 16 interviews to four, chiefly through reduced oversharing and out-of-role expression. Unsupported clinical information remains in one PsyCPG interview (Figure~\ref{fig:app-a-validation-flags}).

\paragraph{Accessible evidence, within a limited validation.} Exact source-code recovery rises from 24/30 to 29/30 at rank one and from 26/30 to 29/30 anywhere, with no reversals (Table~\ref{tab:app-a-diagnosis-pairs}). McNemar probabilities of .063 and .250 reflect few discordant pairs. Recovery measures reference-label accessibility, rather than independent clinical correctness. Evidence is limited to 30 cases, two experts, Persian dialogue, one backbone, and 16 exchanges; it does not isolate individual controls or establish equivalence to real patients or transfer across settings.
