# Supplementary material for: From Dialogue to Diagnostic Hypotheses: Evaluating LLM Agents for Psychiatric Assessment
Source: arXiv:2610.07473 source file (2026-11-06)
Supplement: Supplementary file 24 [file mh-spqf.tex]

% A dedicated full-width form page; prose remains in ACL two-column mode.
\clearpage
\twocolumn[{
\begin{minipage}{\textwidth}
\centering
\includegraphics[width=\textwidth,height=.88\textheight,keepaspectratio]{app_a_mh_spqf.pdf}
\AppendixFigureCaption{MH-SPQF v1.0 in English: all nine items, response anchors, five quality flags, optional comment, and scoring. The study administered the bilingual English/Persian instrument. Item, anchor, and flag wording is reproduced from the frozen form; its instructions are described in the accompanying protocol and omitted here to give the response scale and flags more space.}{fig:app-a-mh-spqf}
\end{minipage}
}]
\clearpage
