# Supplementary material for: From Dialogue to Diagnostic Hypotheses: Evaluating LLM Agents for Psychiatric Assessment
Source: arXiv:2610.07473 source file (2026-11-06)
Supplement: Supplementary file 25 [file section.tex]

\section{PsyCPG: Patient Profile Generation and Simulation}
\label{app:profile}
\label{app:profile-pipeline}

Developing a new patient simulator was not the initial research objective of this work. Our primary aim was to study psychiatric interviewing and diagnostic reasoning, but controlled experiments required a patient counterpart with known clinical evidence, varied conversational behavior, and a stable representation across system comparisons. Direct role-play from a clinical record did not provide sufficient control over how clinical knowledge, personal disposition, and disclosure should enter the conversation. These requirements led us to develop PsyCPG (Psychiatric Case-based Profile Generation).

We regard PsyCPG as a methodological contribution in its own right: a reusable framework for turning clinical cases into configurable psychiatric patient profiles. Its inputs separate the source case and diagnostic reference from cohort-level personality settings, an expert-authored sociocultural catalogue, source-grounded safety constraints, and scheduled interaction challenges. This separation supports reuse with other case collections after compatible input normalization, while making contextual and behavioral settings explicit study choices. A new setting would require adapting those inputs and validating the resulting patients; the present evaluation concerns the Persian profiles and case collection used here.

The contribution is the combined procedure for constructing, inspecting, and using a patient representation, together with evidence about the quality of its simulations. This section first situates that procedure in prior work and derives its design objectives. It then follows generation through the final profile and role-play controls, analyzes the accepted cohorts, and reports the separate expert validation of simulated-patient quality.

\input{sections/appendix/psycpg/01-positioning-design}
\input{sections/appendix/psycpg/02-generation-pipeline}
\input{sections/appendix/psycpg/03-profile-roleplay}
\input{sections/appendix/psycpg/04-cohort-analysis}
\input{sections/appendix/psycpg/05-validation-protocol}
\input{sections/appendix/psycpg/06-validation-results}
