# Supplementary material for: From Dialogue to Diagnostic Hypotheses: Evaluating LLM Agents for Psychiatric Assessment
Source: arXiv:2610.07473 source file (2026-11-06)
Supplement: Supplementary file 26 [file reader-guide.tex]

\twocolumn[{
\section*{Appendix: Reader's Guide}
\label{app:guide}
\begin{minipage}{\textwidth}
\centering\small
\setlength{\tabcolsep}{4pt}
\renewcommand{\arraystretch}{1.02}
\begin{tabularx}{\textwidth}{@{}p{.085\textwidth}>{\raggedright\arraybackslash}Xr@{}}
\toprule
\multicolumn{2}{@{}l}{\textbf{Contents}} & \textbf{Page} \\
\midrule
\textbf{\ref{app:profile}} & \textbf{PsyCPG: Patient Profile Generation and Simulation} & \textbf{\pageref{app:profile}} \\
\hspace*{0.9em}\ref{app:literature-simulation} & \hspace*{0.9em}Related approaches and design goals & \pageref{app:literature-simulation} \\
\hspace*{0.9em}\ref{app:psycpg-generation} & \hspace*{0.9em}Generation, validation, and acceptance & \pageref{app:psycpg-generation} \\
\hspace*{0.9em}\ref{app:fact-contract} & \hspace*{0.9em}Profile representation and role-play boundaries & \pageref{app:fact-contract} \\
\hspace*{0.9em}\ref{app:cohort-construction} & \hspace*{0.9em}Generated cohorts and quality-gate selection & \pageref{app:cohort-construction} \\
\hspace*{0.9em}\ref{app:psycpg-validation-protocol} & \hspace*{0.9em}Simulator-validation protocol and MH-SPQF & \pageref{app:psycpg-validation-protocol} \\
\hspace*{0.9em}\ref{app:psycpg-validation-results} & \hspace*{0.9em}Expert validation results & \pageref{app:psycpg-validation-results} \\
\addlinespace[5pt]
\textbf{\ref{app:psycidra}} & \textbf{PsyCIDRA: Tool Use and Recorded Examples} & \textbf{\pageref{app:psycidra}} \\
\hspace*{0.9em}\ref{app:tool-use} & \hspace*{0.9em}Observed tool use & \pageref{app:tool-use} \\
\hspace*{0.9em}\ref{app:notepad-example} & \hspace*{0.9em}PsyCIRA notepad tool & \pageref{app:notepad-example} \\
\hspace*{0.9em}\ref{app:evidence-interface} & \hspace*{0.9em}PsyDARA diagnosis report structure & \pageref{app:evidence-interface} \\
\addlinespace[5pt]
\textbf{\ref{app:protocol}} & \textbf{Evaluation Instruments} & \textbf{\pageref{app:protocol}} \\
\hspace*{0.9em}\ref{app:instruments} & \hspace*{0.9em}Expert evaluation instruments & \pageref{app:instruments} \\
\hspace*{0.9em}\ref{app:participant-instruments} & \hspace*{0.9em}Participant questionnaires & \pageref{app:participant-instruments} \\
\hspace*{0.9em}\ref{app:aiie-form} & \hspace*{0.9em}AI Interview Examination & \pageref{app:aiie-form} \\
\hspace*{0.9em}\ref{app:aisc-form} & \hspace*{0.9em}AI Safety Check & \pageref{app:aisc-form} \\
\addlinespace[5pt]
\textbf{\ref{app:simulation-results}} & \textbf{Simulated-Patient Experiments: Extended Analysis} & \textbf{\pageref{app:simulation-results}} \\
\hspace*{0.9em}\ref{app:exchange-budget} & \hspace*{0.9em}Interview budget: 16 versus 24 & \pageref{app:exchange-budget} \\
\hspace*{0.9em}\ref{app:simulation-quality} & \hspace*{0.9em}Expert-rated interview quality and safety & \pageref{app:simulation-quality} \\
\hspace*{0.9em}\ref{app:heldout-errors} & \hspace*{0.9em}Held-out errors by diagnostic family & \pageref{app:heldout-errors} \\
\hspace*{0.9em}\ref{app:simulation-confidence} & \hspace*{0.9em}Confidence and rank-1 correctness & \pageref{app:simulation-confidence} \\
\addlinespace[5pt]
\textbf{\ref{app:human-results}} & \textbf{Human-Participant Study: Extended Analysis} & \textbf{\pageref{app:human-results}} \\
\hspace*{0.9em}\ref{app:human-attrition} & \hspace*{0.9em}Participant flow and cohort composition & \pageref{app:human-attrition} \\
\hspace*{0.9em}\ref{app:expert-agreement} & \hspace*{0.9em}Interview quality and safety & \pageref{app:expert-agreement} \\
\hspace*{0.9em}\ref{app:diagnostic-decisions} & \hspace*{0.9em}Diagnostic decisions and code agreement & \pageref{app:diagnostic-decisions} \\
\hspace*{0.9em}\ref{app:human-confidence} & \hspace*{0.9em}Reported support and confidence & \pageref{app:human-confidence} \\
\hspace*{0.9em}\ref{app:experience} & \hspace*{0.9em}Participant-reported experience & \pageref{app:experience} \\
\hspace*{0.9em}\ref{app:resources} & \hspace*{0.9em}Latency and computational resources & \pageref{app:resources} \\
\bottomrule
\end{tabularx}
\AppendixTableCaption{Appendix contents. Bold sections group indented subsections; section and page references are linked.}{tab:appendix-contents}
\end{minipage}
\vspace{10pt}
}]

This appendix brings together methodological details, evaluation materials, and additional results that supplement the main paper. Its purpose is to help readers examine how the studies were conducted and look more closely at their findings. It includes complete evaluation forms and selected examples, but is not a full implementation manual. To keep the appendix focused, we omit exhaustive implementation listings and raw result tables.
\ifdefined\PsyCIDRAReview
The code, prompts, simulation data, expert reviews, and complete result tables are provided with the submission and will be made publicly available with the final version.
\else
The code, prompts, simulation data, expert reviews, and complete result tables are publicly available in \href{https://github.com/PsyCIDRA/PsyCIDRA}{our repository}.
\fi

Section~\ref{app:profile} describes the construction of the simulated patients and includes a sample profile. It also gives the cohort summaries, the complete simulator-validation form, and expert ratings of the resulting interviews.

Section~\ref{app:psycidra} examines observed tool use and timing, and uses recorded examples to clarify the notepad interface and diagnosis report structure.

\newpage
Section~\ref{app:protocol} gives the design rationale and complete forms for interview quality and safety, a brief note on the communication-scale adaptation, and the participant questionnaires.

Section~\ref{app:simulation-results} presents additional analyses of the simulated-patient experiments: the interview-budget comparison, expert ratings of quality and safety, held-out errors by diagnostic family, and the relationship between reported confidence and code correctness.

Section~\ref{app:human-results} follows the human study from participant flow and cohort composition to expert-rated interview quality and safety. It then examines diagnostic decisions, code agreement, and reported confidence before turning to participant experience and recorded latency and token use.
