# Supplementary material for: From Dialogue to Diagnostic Hypotheses: Evaluating LLM Agents for Psychiatric Assessment
Source: arXiv:2610.07473 source file (2026-11-06)
Supplement: Supplementary file 27 [file 01-interview-budget.tex]

\section{Simulated-Patient Experiments: Extended Analysis}
\label{app:simulation-results}
\subsection{Interview budget: 16 versus 24}
\label{app:exchange-budget}
\begin{minipage}{\textwidth}
\centering\small
\setlength{\tabcolsep}{5pt}
\renewcommand{\arraystretch}{1.1}
\input{generated/app_d_budget}
\AppendixTableCaption{The same 53 evaluation profiles under 16- and 24-exchange caps (GPT-5.6 Terra). R1 and coverage are correct counts; tokens are cohort totals in millions, including patient replies, repeated context, and diagnosis.}{tab:app-d-budget}
\end{minipage}
\vspace{6pt}

\begin{minipage}[t]{.48\textwidth}
The longer cap gives no consistent rank-1 benefit. PsyCIDRA remains at 44/53, gains one covered reference, and uses 51\% more tokens. We selected 16 for the human study to limit participant burden and test a brief interview.
\end{minipage}\hfill
\begin{minipage}[t]{.48\textwidth}
The interviews were independently generated.

Future work should adapt interview length and follow-ups without prematurely favoring a diagnosis or reducing the patient's account to isolated symptom checks \citep{vanderheijden-2022-positive-tests,savander-2021-subjective-experiences}.
\end{minipage}
