# Supplementary material for: From Dialogue to Diagnostic Hypotheses: Evaluating LLM Agents for Psychiatric Assessment
Source: arXiv:2610.07473 source file (2026-11-06)
Supplement: Supplementary file 28 [file 02-interview-quality.tex]

\subsection{Expert-rated interview quality and safety}
\label{app:simulation-quality}
\begin{minipage}{\textwidth}
\centering
\includegraphics[width=\textwidth]{app_d_quality_items.pdf}
\AppendixFigureCaption{Expert item means (items: Appendix~\ref{app:instruments}). AIIE has 23 transcripts per interviewer; adapted CCSS-S has 21--23 per item and condition. Item 13 is omitted (one per condition). Missing ratings are excluded.}{fig:app-d-quality-items}
\end{minipage}
