# Supplementary material for: From Dialogue to Diagnostic Hypotheses: Evaluating LLM Agents for Psychiatric Assessment
Source: arXiv:2610.07473 source file (2026-11-06)
Supplement: Supplementary file 29 [file 03-heldout-errors.tex]

\subsection{Held-out errors by diagnostic family}
\label{app:heldout-errors}
\begin{minipage}{\textwidth}
\centering
\includegraphics[width=\textwidth]{app_d_family_confusion.pdf}
\AppendixFigureCaption{Rank-1 family confusion on 81 held-out profiles. Rows are reference families; columns are predicted families. Cells show counts; shading shows row shares on a shared scale.}{fig:app-d-family-confusion}
\end{minipage}
\vspace{2pt}

\begin{minipage}[t]{.48\textwidth}
Family agreement is similar (Direct: 60/81; PsyCIDRA: 61/81), versus 42 and 49 exact-code matches. PsyCIDRA's advantage mainly concerns finer distinctions within families: 12 within-family code misses versus 18 for Direct.
\end{minipage}\hfill
\begin{minipage}[t]{.48\textwidth}
\ifdefined\PsyCIDRAReview
Analysis code and complete simulation results are provided with the submission and will be made publicly available with the final version, enabling researchers to examine individual code substitutions and alternative groupings.
\else
Analysis code and complete simulation results are publicly available in \href{https://github.com/PsyCIDRA/PsyCIDRA}{our repository}, enabling researchers to examine individual code substitutions and alternative groupings.
\fi
\end{minipage}
