# Supplementary material for: From Dialogue to Diagnostic Hypotheses: Evaluating LLM Agents for Psychiatric Assessment
Source: arXiv:2610.07473 source file (2026-11-06)
Supplement: Supplementary file 30 [file 04-confidence.tex]

\subsection{Confidence and rank-1 correctness}
\label{app:simulation-confidence}
\begin{minipage}{\textwidth}
\centering
\includegraphics[width=\textwidth]{app_d_confidence.pdf}
\AppendixFigureCaption{Exact-code rank-1 correctness by reported confidence on the held-out cohort. Bars show within-group proportions; labels give percentages and counts, and $n$ gives group size.}{fig:app-d-confidence}
\end{minipage}
\vspace{6pt}

\begin{minipage}[t]{.48\textwidth}
PsyCIDRA's confidence better separates correct from incorrect first hypotheses in this sample. It reserves ``high'' for five reports, all correct, while Direct's high-confidence group includes 15 errors among 46 reports. PsyCIDRA still makes 19 errors among 60 moderate-confidence reports.
\end{minipage}\hfill
\begin{minipage}[t]{.48\textwidth}
For its intended use as a tool for expert review, this more selective confidence signal may help clinicians prioritize scrutiny. The labels are ordinal, not calibrated probabilities; five high-confidence reports provide limited evidence, and usefulness for expert review remains to be tested.
\end{minipage}
