# Supplementary material for: From Dialogue to Diagnostic Hypotheses: Evaluating LLM Agents for Psychiatric Assessment
Source: arXiv:2610.07473 source file (2026-11-06)
Supplement: Supplementary file 31 [file quality-summary.tex]

\noindent\textbf{\ref{app:simulation-quality}\quad Expert-rated interview quality and safety (continued)}
\vspace{2pt}

\begin{minipage}[t]{.48\textwidth}
\vspace{0pt}
\centering\small
\setlength{\tabcolsep}{4pt}
\renewcommand{\arraystretch}{.95}
\input{generated/app_d_quality_domains}
\AppendixTableCaption{Transcript means across available reviewers; overall scores weight items equally.}{tab:app-d-quality-domains}
\end{minipage}\hfill
\begin{minipage}[t]{.48\textwidth}
\vspace{0pt}
PsyCIRA's clearest gains concern rapport and flow, particularly empathetic validation, responsiveness, and summarization. Diagnostic inquiry is similar; risk recognition is slightly lower.

Ratings cover 46 transcripts from 30 selected profiles and 60 expert reviews. AISC flags one PsyCIRA transcript for crisis neglect and none for Direct; these small counts do not establish a safety difference.
\end{minipage}
