# Supplementary material for: From Dialogue to Diagnostic Hypotheses: Evaluating LLM Agents for Psychiatric Assessment
Source: arXiv:2610.07473 source file (2026-11-06)
Supplement: Supplementary file 32 [file section.tex]

% Deliberate page bands preserve subsection order without one page per subsection.
\twocolumn[{
\input{sections/appendix/simulation-results/01-interview-budget}
\vspace{4pt}
\input{sections/appendix/simulation-results/02-interview-quality}
}]
\clearpage
\twocolumn[{
\input{sections/appendix/simulation-results/quality-summary}
\vspace{2pt}
\input{sections/appendix/simulation-results/03-heldout-errors}
}]
\clearpage
\twocolumn[{
\input{sections/appendix/simulation-results/04-confidence}
}]
